# Supplementary material for: MOA-2020-BLG-135Lb: A New Neptune-class Planet for the Extended MOA-II Exoplanet Microlens Statistical Analysis
Source: arXiv:2204.03672 source file (2025-04-14)
Supplement: Supplementary file 1 [file aastex63_additional_journal_abbreviations.tex]

\newcommand\cse{\ref@jnl{CSE}}%     %  Computing In Science Engineering %%CR Added
